# Supplementary material for: Spontaneous surface flux pattern in chiral p-wave superconductors - revisited
Source: arXiv:1710.07998 ancillary file (2018-03-25)
Supplement: Supplementary file 1 [file flux_pattern_supp.pdf]

# Supplemental Material for
# Spontaneous surface flux pattern in chiral $p$-wave superconductors

Sarah B. Etter,[1] Adrien Bouhon,[2] and Manfred Sigrist[1]

[1] *Institute for Theoretical Physics, ETH Zurich, 8093 Zurich, Switzerland*
[2] *Department of Physics and Astronomy, Uppsala University, Box 516, SE-751 20 Uppsala, Sweden*

(Dated: March 25, 2018)

In this Supplemental Material we provide the actual numerical values for the boundary conditions for each surface type $s$ in Sec. I, and the full numerical results of the flux pattern for all surface types $s$ and all ratios $K_1/K_2$ in Sec. II.

## I. VALUES OF THE BOUNDARY CONDITIONS FOR THE SURFACE TYPES

The spontaneous magnetic flux pattern is computed for 31 surface types $s \in \{0, \ldots, 30\}$ indicated by the black dots in Fig. 2 in the main paper. The actual numerical values for the corresponding $g_i$ and $T_{ci}^{\text{eff}}$, defined in Eqs. (13) and (14) of the main paper, are summarized below in Table I.

As shown in Fig. 2 in the main paper, the range B follows a line $g_3 = 2g_0 - g_1$, with $g_0 \to \infty$. The value of $g_0$ does not have to be specified, because we explicitly set $\eta(R) = 0$ at the surface for the corresponding component(s) of the order parameter in these cases. However, a cut-off has to be introduced (i.e. the value just before $g_0$). From the analysis of the extrapolation lengths the applicability of the chosen cut-off was confirmed, see Fig. 4 in the main paper. To exclude the origin, the range D follows $g_3 = 2g_m - g_1$ with $g_m = g_3(s = 0) = 0.25$.

## II. FULL NUMERICAL RESULTS OF THE FLUX PATTERN

In Figure 1 below, the full numerical results of the detailed shape of the magnetic flux pattern are provided as a chart of density plots for each surface type $s$ and each ratio $K_1/K_2$. The same color scheme is used as for Figs. 5 and 6 in the main paper.

Selected quantities extracted from these results are discussed in Fig. 7 in the main paper, such as the current direction at the surface, the total flux, and a Fourier analysis.

TABLE I. The numerical values of the boundary conditions for the 31 surface types $s$ indicated in Fig. 2 in the main paper (black dots). The value of $g_0$ does not have to be specified, because for $T_c^{\text{eff}}/T_c = 1 - 2g_0$ the corresponding order parameter component is set to zero explicitly at the surface, $\eta(R) = 0$, as explained above.

| range | $s$ | $g_1/(\xi_0 a T_c)$ | $g_3/(\xi_0 a T_c)$ | $T_{c\perp}^{\text{eff}}/T_c$ | $T_{c\parallel}^{\text{eff}}/T_c$ | surface type |
|---|---|---|---|---|---|---|
| | - | 0 | 0 | 1 | 1 | virtual boundary |
| A | 0 | 0.25 | 0.25 | 0.5 | 1 | |
| A | 1 | 0.5 | 0.5 | 0 | 1 | |
| A | 2 | 0.75 | 0.75 | -0.5 | 1 | |
| A | 3 | 1 | 1 | -1 | 1 | |
| A | 4 | 1.25 | 1.25 | -1.5 | 1 | |
| A | 5 | 1.75 | 1.75 | -2.5 | 1 | |
| A | 6 | 3 | 3 | -5 | 1 | |
| A | 7 | 5.5 | 5.5 | -10 | 1 | |
| | **8** | $g_0$ | $g_0$ | $1-2g_0$ | 1 | specular |
| B | 9 | $g_0+0.125$ | $g_0-0.125$ | $1-2g_0$ | 0.75 | |
| B | 10 | $g_0+0.25$ | $g_0-0.25$ | $1-2g_0$ | 0.5 | |
| B | 11 | $g_0+0.5$ | $g_0-0.5$ | $1-2g_0$ | 0 | |
| B | 12 | $g_0+0.75$ | $g_0-0.75$ | $1-2g_0$ | -0.5 | |
| B | 13 | $g_0+1$ | $g_0-1$ | $1-2g_0$ | -1 | |
| B | 14 | $g_0+1.25$ | $g_0-1.25$ | $1-2g_0$ | -1.5 | |
| B | 15 | $g_0+1.75$ | $g_0-1.75$ | $1-2g_0$ | -2.5 | |
| B | 16 | $g_0+3$ | $g_0-3$ | $1-2g_0$ | -5 | |
| B | 17 | $g_0+5.5$ | $g_0-5.5$ | $1-2g_0$ | -10 | |
| | **18** | $2g_0$ | 0 | $1-2g_0$ | $1-2g_0$ | full pair-breaking |
| C | 19 | 11 | 0 | -10 | -10 | |
| C | 20 | 6 | 0 | -5 | -5 | |
| C | 21 | 3.5 | 0 | -2.5 | -2.5 | |
| C | 22 | 3 | 0 | -2 | -2 | |
| C | **23** | 2.5 | 0 | -1.5 | -1.5 | vanishing total flux |
| C | 24 | 2 | 0 | -1 | -1 | |
| C | 25 | 1.5 | 0 | -0.5 | -0.5 | |
| C | 26 | 1 | 0 | 0 | 0 | |
| C | 27 | 0.5 | 0 | 0.5 | 0.5 | |
| D | 28 | 0.4375 | 0.0625 | 0.5 | 0.625 | |
| D | 29 | 0.375 | 0.125 | 0.5 | 0.75 | |
| D | 30 | 0.3125 | 0.1875 | 0.5 | 0.875 | |

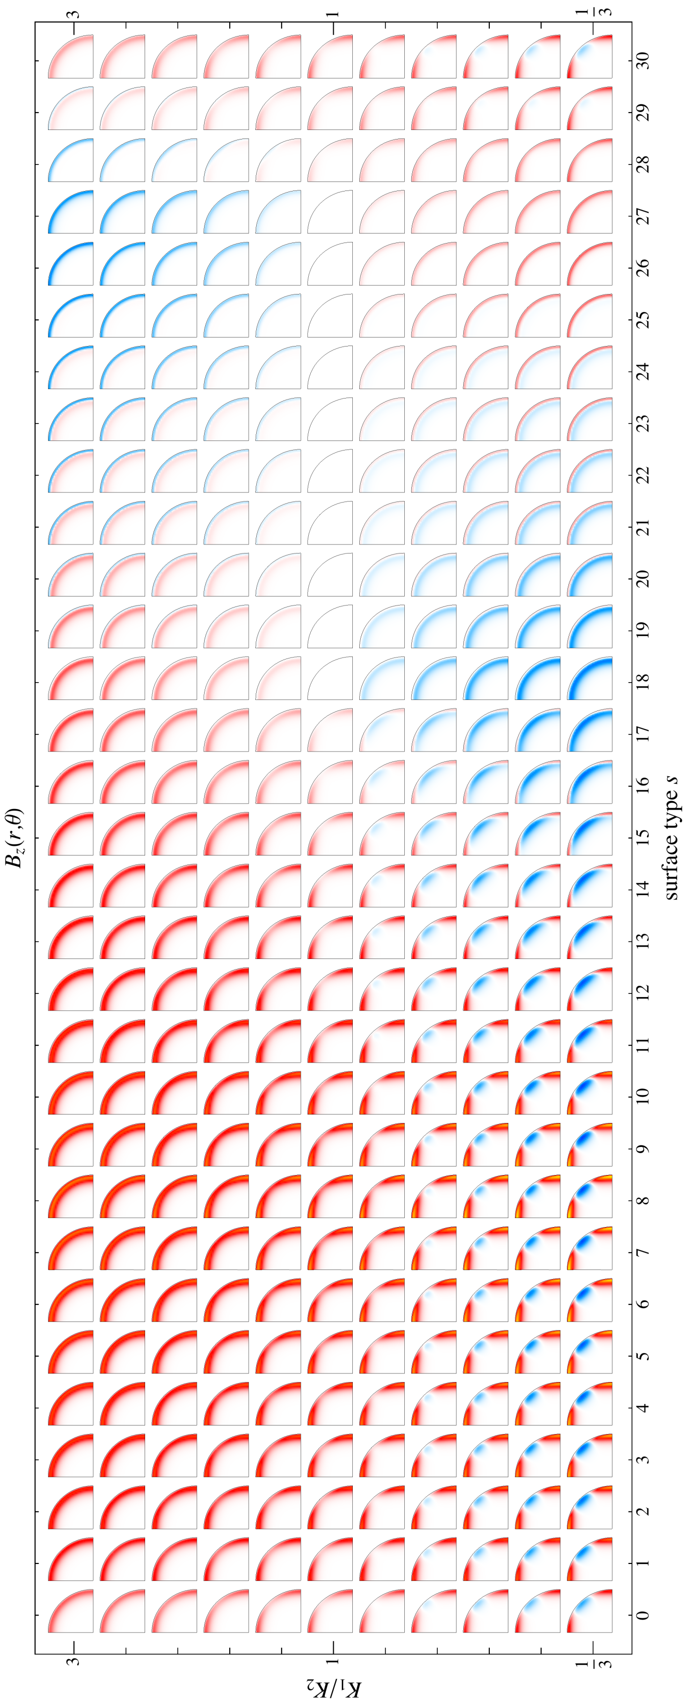


FIG. 1. Full numerical results for the flux pattern $B_z(r,\theta)$ arranged in a chart of the ratio $K_1/K_2$ versus the surface type $s$ with the same color scheme as for Figs. 5 and 6 in the main paper.
